# Supplementary material for: TALUS: Reinforcing TEE Confidentiality with Cryptographic Coprocessors (Technical Report)
Source: arXiv:2306.03643 source file (2023-06-06)
Supplement: Supplementary file 1 [file requirementAnalysis_Appendix.tex]

%!TEX root=../main.tex

In this section, we document how the coprocessors and TEEs performs against the requirements and objectives defined in \Cref{objDefinition} and \Cref{sec:additional-objectives}. 
\Cref{tab:systematizationRequirements} and \Cref{tab:systematizationObjectives} is populated for each of the candidates based on the analysis done in this section. 

\begin{figure}[t]
	\centering
	\begin{subfigure}[b]{\hsize}
		\centering
		\includegraphics[width=0.8\hsize]{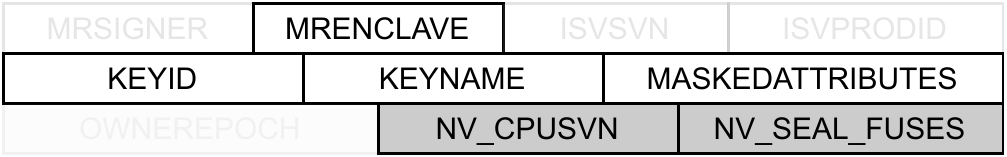}
		\caption{\footnotesize \lstinline{EREPORT} key derivation material}
		\label{fig:usecasesealkeykdm}
	\end{subfigure}
	\hfill
	\begin{subfigure}[b]{\hsize}
		\centering
		\includegraphics[width=0.8\hsize]{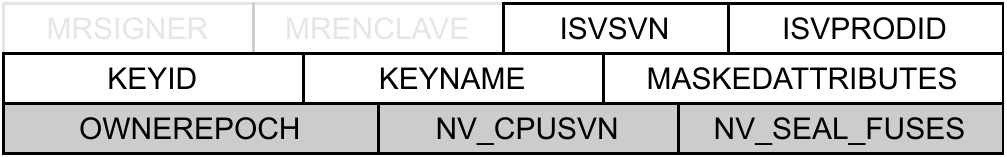}
		\caption{\footnotesize \lstinline{EINITTOKEN} key derivation material}
		\label{fig:usecaseeinittokenkdm}
	\end{subfigure}
	\hfill
	\begin{subfigure}[b]{\hsize}
		\centering
		\includegraphics[width=0.8\hsize]{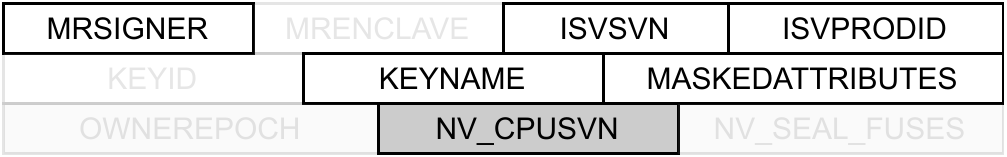}
		\caption{\footnotesize \lstinline{PROVISIONING KEY} key derivation material}
		\label{fig:usecaseprovisioningkeykdm}
	\end{subfigure}
	\caption{\ournameplain key derivation material example}
	\label{fig:keyderivationmaterial}
\end{figure}

\begin{figure}[t]
		\centering
		\includegraphics[width=\hsize]{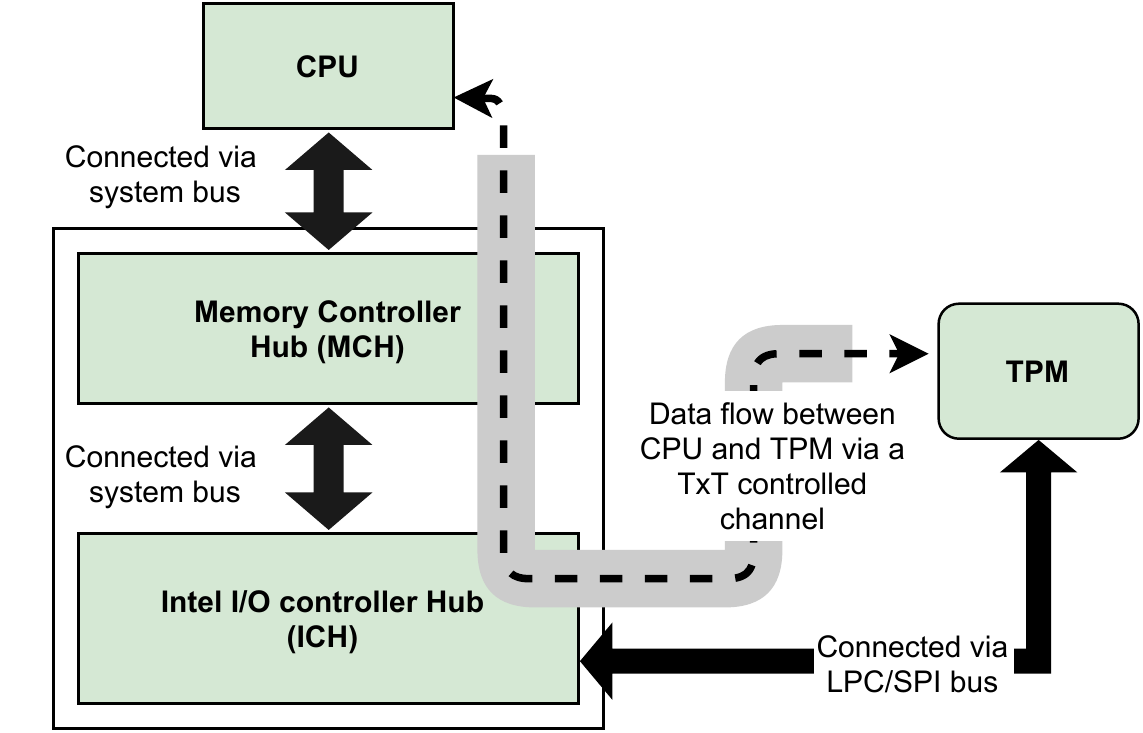}
		\caption{Communication between CPU and \tpm. 
		Data flows through the Memory Controller Hub (MCH), Intel I/O Controller Hub (ICH), system bus, and LPC/SPI bus, all controlled by \txt. 
		This channel is end-to-end encrypted~\cite{Futral2013, TPM2Cmd}.} 
		\label{fig:tpmconn}
\end{figure}

\subsubsection{AMD PSP}
\label{sumPSP}

AMD's Platform Security Processor (PSP) often also known as AMD Secure Processor is a coprocessor integrated into the processor package. 
It provides co-processing support to safeguard the secrets used for the lifecycle of AMD SEV. 
Being part of the processor package makes it easier to establish a secure communication channel with the processor (\textbf{PSP CC1: \yes}). 
However, the PSP communicates through MMIO registers (mailbox registers) which introduces a dependency on external insecure buffers (\textbf{PSP CC2: \scros}), making it hard to guarantee security against a \textit{MMIO mapping attack}~\cite{ZhGlNeMc2012}.

PSP is solely used to serve SEV and platform integrity through secure boot (\textbf{PSP VC: \scros}). 
It can distinguish between different requests originated from SEV (\textbf{PSP HC: \yes}). 
However, the command buffer used for PSP commands allocated and controlled by the x86 system software or the OS makes it dependent on the untrusted OS (\textbf{PSP SP2: \yes}). 
PSP employs strict hardware isolation for its security co-processing (\textbf{PSP SP1: \yes}).

To our knowledge, PSP does not provide any source of secure clock but uses the base board clock if required (\textbf{PSP TCB2: \scros}). 
AMD PSP does not employ any kind of non-volatile storage that can be used to store cryptographic secrets.
The SEV firmware is responsible for guaranteeing the confidentiality and integrity of secrets (\textbf{PSP SSC1: \scros}). 
PSP does not provide any kind of rollback protection (\textbf{PSP SSC2: \scros}). 
We are unable to find any available command or API that offers any types of flexible access control policies (\textbf{PSP TCB1: \unknown}).

\subsubsection{AMD SEV}
\label{sumSEV}

The AMD Secure Encrypted Virtualization is an application-processor-based TEE encrypting the memory contents of VMs. 
The encrypted states of the VMs are located in main memory.
The content of VMs is only decrypted when it loaded into the processor. 
SEV still relies on external insecure buffers, such as caches (\textbf{SEV CC2: \scros}). 

SEV uses PSP as a coprocessor and often communicates with it for isolated cryptographic coprocessoring.
However, PSP is registered as MMIO device and uses MMIO registers for communication (\Cref{objPSP}), resulting in an insecure communication channel (\textbf{SEV CC1: \scros}). 

The SEV firmware (which is part of the processor firmware) functions as the generator of the access control tokens for the VM communication. 
PSP ensures the availability of a trusted entity for access control in case of horizontal access control (\textbf{SEV HC: \yes}). 
However, SEV does not offer any service to the other software on the platform (\eg OS or applications) to access PSP in a secure manner % removes the need of a trusted entity for vertical access control
(\textbf{PSP VC: \scros}). 

SEV runs on the processor and thus shares microarchitectural elements with untrusted software (\textbf{SEV SP1: \kinda}). 
SEV heavily depends on the hypervisor which is not part of its TCB (\textbf{SEV SP2: \scros}). 

SEV depends on the mainboard clock as there is no other clock source available (\textbf{SEV TCB2: \scros}). 
SEV SNP, \ie SEV with the secure nested paging extion, provides protection against firmware rollback but shows no evidence providing protection against virtual machine state roll back attack as it provides no secure storage capability (\textbf{SEV SSC2: \kinda} and \textbf{SEV SSC1: \scros}). 
SEV provides a limited list of APIs to the VM and does not offer much flexibility around this APIs (\textbf{SEV TCB1: \scros}).

\subsubsection{Intel PTT with Intel CSME}
\label{sumPTT}

Intel PTT~\cite{intelPTT2014} is Intel's implementation of a firmware \tpm compliant with the TCG TPM 2.0~\cite{TPM2Arch} and Microsoft fTPM~\cite{Raj2016} standard.
Intel PTT runs inside Intel CSME~\cite{intelCSME2020}. 
PTT uses the isolated execution environment powered by a 32-bit processor based on the Intel 486 architecture with a small dedicated SRAM (\textbf{PTT SP1: \yes}). 
CSME employs its own TCB OS with its own security ring, completely segregated from the platform security.
However, the command buffer for PTT is configured by untrusted software such as the OS (\textbf{PTT SP2: \yes}). 

CSME offers trusted read-only memory for the CSME root of trust. 
PTT uses CSME's trusted storage to store its endorsement key, storage root key, or other root keys. 
However, recently found attacks CVE-2018-3659, CVE-2018-3643 \cite{csmeATTACK2018} and CVE-2019-0090, CVE-2020-0566~\cite{csmeATTACK2019} on CSME compromise all its use cases. 
User secrets protected by Intel PTT are compromised (\textbf{PTT SSC1: \scros}) and Intel recommended to use \htpm instead or PTT. 
These CVEs remove trust from Intel Dynamic Allocation Loader (DAL) and thus also the secure counter and rollback protection (\textbf{PTT SSC2: \scros}). 

PTT's use cases are limited to the OS and hardware around measured boot, platform attestation and disk encryption.
PTT does not offer support to ring 3 software including \sgx enclaves. 
Hence, it does not require to offer flexible policies similar to \sgx \texttt{EGETKEY} or TPM EAP (\textbf{PTT TCB1: \scros}). 
PTT does not employ horizontal (\textbf{PTT HC: \scros}) or vertical (\textbf{PTT VC: \scros}) access control. 
CSME offers a real-time clock that can be used for monotonic counters. 
However, they are limited to CSME use cases. 
PTT does not offer any service to its client (\eg OS or Hardware) that requires a clock (\textbf{PTT TCB2: \kinda}). 

CSME is housed in the Platform Control Hub (PCH) which is connected to the processor via DMI and employs no encryption to secure the communication (\textbf{PTT CC1: \scros}). 
Although PTT uses the isolated execution environment provided by CSME, it is unknown if it relies on any insecure external buffers (\textbf{PTT CC2: \unknown}).

\subsubsection{Google Titan}
\label{sumGoogletitan}
Google has introduces its own security hardware called Titan M2 \cite{titanM}. 
It is designed and developed using a RISC-V processor combined with its own memory~\cite{titanM21} offering strict hardware isolation (\textbf{Titan SP1: \yes}). 
The goal of Titan with Android keymaster~\cite{AndroidKeystore} is to keep the key material secure with no possibility of extracting it from the hardware~\cite{AndroidKeystoreSecurityFeature}. 
The Titan backed keystore does not release keys to the system (\textbf{Titan SP2: \yes}). 
Hence, the Titan supported systems are likely free from microarchitectural or side-channel attacks as the keys are never available in microarchitectural buffers (\textbf{Titan CC2: \yes}).

Titan provides secure storage for the keys it generates or imports for its client (\textbf{Titan SSC1: \yes}). 
This storage can be used to store secure counter for rollback protection too. 
However, we are unaware of existence of such counters (\textbf{Titan SSC2: \kinda}).  

To access a key, a client must provide the password related to the key. 
This protects the access control to the key and key material but lacks flexibility (\eg flexibility offered by TPM EAP) (\textbf{Titan TCB1: \kinda}). 
Titan does not employ any kind of horizontal (\textbf{Titan HC: \scros}) or vertical (\textbf{Titan VC: \scros}) access control. 
Moreover, Titan provides no secure clock service to its client (\textbf{Titan TCB2: \scros}).

Lastly, it is unknown if Android or the underlying hardware employs any kind of security around the communication channel to Titan chip (\textbf{Titan CC1: \scros}). 

\subsubsection{Intel SGX}
\label{sumSGX}
Intel \sgx provides a general-purpose isolated code execution environment on Intel platforms. 
While \sgx provides isolation on an architectural level, it fails to ensure isolation on the microarchitectural level. 
As microarchitectural elements, such as caches, are shared between the secure enclaves and the untrusted systems (\textbf{\sgx CC2: \scros}), side-channel attacks can observe the shared microarchitectural state~\cite{Schwarz2020How,vanbulck2020phd}. 
Additionally, the recent discovery of transient-execution attacks~\cite{Lipp2018,Kocher2018,Bulck2018,Schwarz2019,ridl2019,VanBulck2020LVI} violates the confidentiality guarantee of \sgx. 
\sgx uses the PTT (a firmware TPM by Intel) for certain use-cases. 
PTT is housed inside the CSME and can be connected via DMI interface without any security around this channel (\textbf{\sgx CC1: \scros}). 
In addition, PTT suffers from recently found attacks CVE-2018-3659, CVE-2018-3643~\cite{csmeATTACK2018} and CVE-2019-0090, CVE-2020-0566~\cite{csmeATTACK2019} that can compromise all its use cases (see \Cref{objPTT}). 
In practice, \sgx fails the objective of strict hardware isolation (\textbf{SGX SP1:~\scros}). 

Although the OS is not part of the trusted computing base of \sgx, \sgx is not OS-agnostic (\textbf{\sgx SP2:~\scros}). 
The OS is responsible for creating and managing enclaves. 
It allocates memory for the enclaves, manages address-translation structures for enclave memory, and copies data and code into the enclave~\cite{McKeen2016ISG}. 
All the enclave initialization actions by the OS are securely logged by SGX and are verified on enclave launch to ensure launch-time enclave integrity. 
As Intel SGX needs the OS for memory management, \sgx enclaves can be interrupted by the OS, enabling an additional attack surface, \eg controlled-channel attacks~\cite{controlledsidechannel} or precise execution control of the enclave~\cite{sgxstep2017}. 

Intel \sgx is not equipped with a secure source of clock but receives the clock information from the system clock, which can be modified by the untrusted OS. 
Moreover, the OS can distort an enclave's perception of time through interrupts~\cite{Huang2021aion} (\textbf{\sgx TCB2:\scros}). 
In \sgx, support for counters depends on the Platform Service Enclave and Intel ME, which often are not available in \sgx production deployments, and already deprecated~\cite{intelCounter} (\textbf{\sgx SSC2: \kinda}). 
Moreover, these counters can be simply reset by reinstalling the SGX platform software~\cite{MateticAKDSGJC17}. 
As \sgx stores counters inside the BIOS flash storage, they do not persist across system resets~\cite{MateticAKDSGJC17} (\textbf{\sgx SSC1:\scros}). 

A desirable objective is support for flexible access-control policies for secure storage. 
\sgx allows enclaves to implement custom authorization logic and use the result as input to the key derivation with \lstinline{EGETKEY}, making the key \emph{generation} similarly flexible as using \tpm EAP but relying on correct implementation by the enclave developers (\textbf{\sgx TCB1: \kinda}).
Additionally, \sgx does not offer any support to software other than enclaves and requires no vertical access control mechanism (\textbf{\sgx VC: \scros}). 
However, for horizontal access control, \sgx identifies enclaves using their identification stored in \textit{SECS} (\textbf{\sgx HC: \yes})~\cite{CostanD2016}.

\subsubsection{Hardware TPM}
\label{sumTPM}
\tpm by the Trusted Computing Group is the most widely deployed trusted computing technology on commodity platforms, currently in version 2.0~\cite{TPM2Spec}. 
TPM offers strict hardware isolation by exporting its execution environment to a secure coprocessor chip.
This low-end 32-bit coprocessor also has access to a small RAM (\textbf{TPM SP1: \yes}) and NV-storage. 
The NV-storage implemented inside the TPM chip offers complete confidentiality and integrity of storage of secrets (\textbf{TPM SSC1: \yes}). 
\tpm uses handles (random 32-bit values) to reference different types of \tpm-internal managed resources~\cite{TPM2Struct,TPM2HandleNLocality} such as keys, data blobs, authorization sessions, NVM regions, %permanent \tpm locations 
and PCRs. 
For instance, when a \tpm client generates a cryptographic key with \tpm, \tpm returns a \textit{key handle} instead of the key itself, which the client has to use for, \eg signing or decryption with this key through the \tpm. 
The key handle itself is not security-sensitive since to use the referenced key in a \tpm command, the client has to prove its access rights to that key through \textit{Command Authorization} by using Extended Authorization Policy (EAP).
The aforementioned storage can be used to implement secure counters which also can provide protection against version rollback attacks for both system and third party software, and hardware (\textbf{TPM SSC2: \yes}).

TPM employes both EAP and Locality to provide access control for both access request from same security ring (\textbf{TPM HC: \yes}) and requests across security rings (\textbf{TPM VC: \yes}) respectively. 
These access-control policies are very flexible and can be implemented from hardware, OS, to third-party software.
They take advantage of the TPM to secure their secrets or offload their secure execution away from application processor (\textbf{TPM TCB1: \yes}). 
TPM also implements its own secure source of clock (available at 33 MHz granularity) that makes it independent of untrusted system clock for temporal attestation and commands (\textbf{TPM TCB2: \yes}).

Typically, a \tpm is available as a hardware chip soldered onto the mainboard, connected traditionally via the Low Pin Count (LPC) bus or on newer platforms via the SPI bus, making it available through memory-mapped I/O (MMIO) registers protected by the chipset. 
Additionally, a hardware-controlled channel connects the CPU to the \tpm through the Memory Controlled Hub and I/O Controller Hub \cite{ioControllerDataSheet}. 
This channel is also known as the programmed I/O channel. 
By specification~\cite{Futral2013, TPM2Cmd}, the hardware channel between CPU and \tpm is end-to-end encrypted to protect against bus sniffing attacks.
TPM offers end-to-end encryption to secure the communication channel between the processor and TPM. 
TPM 2.0 parameter encryption helps to encrypt the parameter portion of the command to safeguard from other untrusted software (\textbf{TPM CC1: \yes}). 
As the application processor heavily depends on cache and other microarchitectural buffers, the encrypted channel with the TPM helps protecting the communication from cache and other microarchitectural attacks (\textbf{TPM CC2: \yes}). 
Software can initiate secure and encrypted session communication with the \tpm which removes the dependency on untrusted software (\textbf{TPM SP2: \yes}).  

%\subsection{Discussion on Systematization}\notem{not sure if we need this subsection}
%
%From \Cref{tab:systematizationRequirements} and \Cref{tab:systematizationObjectives}, it is evident that for a TEE to function in a hostile platform, a coprocessor is required. 
%Otherwise, the protection of the TEE itself can be compromised. 
%There are major efforts available to create such combination of coprocessor and TEE (\eg AMD SEV with AMD PSP, TrustZone with Titan M2, or Intel \sgx with Intel PTT). 
%However, most combinations still contains security problems due to their design. 
%With \ourname, we present a symbioses of a TEE and a coprocessor, which satisfies all the requirements and additional objectives described in \Cref{objDefinition}. 
%We use \tpm as the coprocessor due to its resilience against a rich set of vulnerabilities and its conformity with a wide range of security technologies and \sgx as the TEE technology due to its wide availability with Intel processor and its open-source implementation through QEMU-SGX \cite{qemuSGX} and KVM-SGX \cite{kvmSGX}. 
%We also believe that this symbiosis can be ported to safeguard other TEEs on other platforms. %the objectives from \Cref{tab:systematizationRequirements} and \Cref{tab:systematizationObjectives} can serve as the standards that such combinations should abide-by.

\subsubsection{ARM TrustZone}
\label{sumArmtrustzone}

TrustZone~\cite{armTZ} is a processor technology that creates a curtained execution environment running on the application processor. 
It segments execution on the application processor into a secure world and non-secure world.
TrustZone implements restrictions on how the non-secure world interacts with the secure world. 
TrustZone also employs its own TEE OS to not depend on the rich OS (\textbf{TrustZone SP2: \scros}). 
However, TrustZone is vulnerable to microarchitectural attack as it depends on external buffers~\cite{RyanCCS19, ARMageddon2016} shared with the non-secure world (\textbf{TrustZone CC2: \scros}). 
Dependencies on the external buffers also reduce the hardware isolation (\textbf{TrustZone SP1: \scros}).
The communication channel with the processor is not secured (\textbf{TrustZone CC1: \scros}).

TrustZone does not offer any secure storage facility. 
Manufacturer, \eg Microsoft, implement RPMB-based storage to store counters and fuses for other secrets such as device specific OEM keys. 
However, this storage is only available to system software (\textbf{TrustZone SSC1: \kinda}). 
Additionally, TrustZone does not offer secure counter or rollback protection~\cite{armTZrollback} for the platform or software (\textbf{TrustZone SSC2: \scros}).

TrustZone does not implement any separate secure clock but uses the mainboard clock that is shared with other untrusted software (\textbf{TrustZone TCB2: \scros}).
TrustZone allows manufacturers to implement trustlets that can run inside the TrustZone.
Application from the rich OS can communicate through the standardized gateway communication APIs. 
TrustZone does not add any special flexibility on the access policies to the trustlets (\textbf{TrustZone TCB1: \scros}). 
Manufacturers and developers have to implement their own access control mechanism to safeguard their secrets residing inside TrustZone. 

Being a processor technology, TrustZone has the capability to distinguish between calls generated between different trustlets (\textbf{TrustZone HC: \yes}), but fails to distinguish between application calls originated from the rich OS (\textbf{TrustZone VC: \kinda}). 
TrustZone only can understand whether the call originated from the rich OS or TEE OS. 

\subsubsection{Apple T2 Security}
\label{sumT2}

Apple implemented the T2 security chip~\cite{t2APPLE} to bring isolated secure co-processing to its platform to support Apple Secure Enclave~\cite{secureEnclaveAPPLE}. 
The T2 chip offers secure boot that ensures the integrity of the entire Apple platform. 
However, Apple offers no protection to the communication channel between application processor and the T2 chip (\textbf{T2 CC1: \scros}). 
T2 protects all the necessary cryptographic keys to implement secure storage for FileVault and secure boot. 

T2 does not release keys to the application processor but the application processor sends command to the T2 chip. 
Hence, there is no key leakage from the external buffers (\textbf{T2 CC2: \yes}). 
Apple implements T2 the functionality with strict hardware isolation (\textbf{T2 SP1: \yes}). 
T2 requires no involvement of any untrusted software (\textbf{T2 SP2: \scros}). 

The T2 chip supports a very limited numbers of usecases and offers no support for non-Apple entities (\textbf{T2 VC: \scros}).
Hence, while the confidentiality and integrity of the T2 storage is available, third party code in the TEE cannot utilize it (\textbf{T2 SSC1: \yes}). 
T2 implements secure rollback protection only to the firmware, resulting in a limited counter support and rollback protection (\textbf{T2 SSC2: \yes}). 
It is unknown how T2 controls system access to the stored secrets (\textbf{T2 HC: \unknown}).

Apple T2 does not offer any secure clock mechanism to the platform (\textbf{T2 TCB2: \scros}).
Furthermore, it does not offer any support to third party code for flexible policies on command and response (\textbf{T2 TCB1: \scros}).

\subsubsection{Microsoft Pluton}
\label{sumPluton}

After fTPM, Microsoft's newest contribution to the trusted-computing sphere is the Pluton security chip~\cite{msPluton}, integrated with the application processor. 
Pluton will be used widely with Microsoft devices and their Azure cloud platform. 

According to Microsoft, Pluton is fully compliant with the TCG TPM 2.0~\cite{TPM2Arch} specification. 
It uses a dedicated ARM M4 processor with \SI{128}{\kilo\byte} of \textit{Tightly Coupled Memory} (TCM) and \SI{64}{\kilo\byte} bootloader ROM \cite{AzureSphere}.
This configuration can provide an isolated hardware execution environment (\textbf{Pluton SP1: \yes}). 
However, it is unknown how confidentiality and integrity of the communication channel is ensured (\textbf{Pluton CC1: \unknown}). 
It is also unknown how the Pluton device is exposed to the platform (\eg as MMIO device) or if any untrusted software dependency is required (\eg preparing the command buffer) to perform actions on Pluton (\textbf{Pluton SP2: \unknown}). 
While it is still unknown how Pluton communicates with the application processor (\eg via DMI interface), we believe that Microsoft can implement custom protocols to communicate with Pluton without using any untrusted buffer (\textbf{Pluton CC2: \unknown}).

As Pluton is fully compliant with a TPM 2.0 device, we believe it is feasible to equip Pluton with both Locality and EAP to support vertical access control (\textbf{Pluton VC: \yes}) and horizontal access control (\textbf{Pluton HC: \yes}). 
With Locality and EAP implemented, it Pluton can also provide flexible policies (\textbf{Pluton TCB1: \yes}).

The Pluton processor does not have a dedicated clock but receives clock frequency from the processor clock (the processor MT3620 is equipped with a \SI{36}{\kilo\hertz} real-time clock). 
However, it is unclear if this clock can be manipulated by untrusted software (\textbf{Pluton TCB2: \kinda}). 

Pluton does not offer any secure storage facility other than programmable fuses to store platform specific cryptographic secrets (\textbf{Pluton SSC1: \kinda}). 
These fuses can be used to store counters to provide rollback protection. 
However, it is doubtful how much this protection can be extended beyond the platform (\textbf{Pluton SSC2: \kinda}). 

\subsubsection{Firmware TPM}
\label{sumfTPM}

Unlike Intel PTT, a firmware TPM is a \tpm software running on the application processor. 
A good example of such a \tpm is Microsoft's fTPM~\cite{Raj2016} implementing the TPM on top of ARM TrustZone.
In a desktop or server environment, such TEEs are unavailable.
Firmware TPMs running on the application processor in parallel to other untrusted processes removes the possibilities of having a secure channel with the processor (\textbf{fTPM CC1: \scros}).
Futhermore, such a firmware TPM also depends on insecure microarchitectural buffers (\textbf{fTPM CC2: \scros}) and cannot offer strict hardware isolation for its execution environment (\textbf{fTPM SP1: \scros}).

If implemented according to the TPM 2.0 specifications from TCG~\cite{TPM2Arch, TPM2Cmd} offering all capabilities of TPM EAP, a firmware TPM supports access tokens (generated on the basis of callee policies) (\textbf{fTPM HC: \yes}). 
If implemented, a firmware TPM can respect the hierarchy of the security levels and can distinguish calls between them (\textbf{fTPM VC: \yes}). 
An implementation of locality and EAP helps an fTPM to provide flexible policies to the client (\textbf{fTPM TCB1: \yes}).

The fTPM in general does not employ any secure storage.
Microsoft fTPM implements a secure storage through a combination of encryption with fused keys, device UUID, and Replay Protected Memory Block (RPMB) with authenticated writes and write counters. 
We believe that this approach can be implemented (only by the manufacturer) with general fTPM (\textbf{fTPM SSC1: \yes}), which is also used to provide secure counter and rollback protection to client (\textbf{fTPM SSC2: \yes}). 

Due to absence of isolated hardware, an fTPM implementation always depends on the system clock (\textbf{fTPM TCB2: \scros}). 
If locality is implemented, different paging regions are available for different security levels to communicate with the \tpm. 
This make an fTPM independent of untrusted software for communication (\textbf{fTPM SP2: \scros}), but only manufacturers can enable this feature.

\subsubsection{RISC-V Keystone Enclaves}
\label{sumRiscvkeystone}

Keystone~\cite{keystone2020} is the first open-source framework for building enclave-type TEEs similar to Intel \sgx on the RISC-V platform. 
Similar to \sgx, Keystone also runs on the application processor and depends on external buffers such as the cache (\textbf{Kystone CC1: \scros}). 
Keystone is designed on SiFive's mainboard equipped with a FU540 module. 
This module employs \textit{waymasking}, a way to implement cache partitioning with the help of a \textit{Security Monitor} (SM). 
\textit{Waymasking} helps segregating enclave content from untrusted software content but does not provide any security from other enclaves if they behave maliciously (\textbf{Keystone CC2: \scros}) and solely depends on formal verification of enclave code.

Keystone does not provide any protection against attacks such as Foreshadow~\cite{Bulck2018} or Spectre~\cite{Kocher2018} as Keystone does not provide strict hardware isolation (\textbf{Keystone SP1: \scros}). 
Keystone does not depend on the OS for page management, as Keystone enclaves have their own runtime.
However, it depends on the SM which is considered secure by Keystone, although it does not provide protection from microarchitectural attacks (\textbf{Keystone SP2: \kinda}).
 
Keystone hints that it can support sealed storage, trusted timers, and rollback protection.
However, it is unclear if Keystone really provides these functionalities~\cite{keystoneGithub} (\textbf{Keystone SSC1, SSC2, TCB2: \scros}). 
It is also unclear to what extent Keystone provides flexibility with its policies to enclave developers (\textbf{Keystone TCB1: \scros}). 
Additionally, similar to \sgx, Keystone does not offer any support to software other than enclaves and requires no vertical access control mechanism (\textbf{\sgx VC: \scros}). 
However, Keystone identifies enclaves using their identification (\textbf{\sgx HC: \yes}).

%%% Local Variables:
%%% mode: latex
%%% TeX-master: "../bare_conf"
%%% End:
